# Supplementary material for: UFNRec: Utilizing False Negative Samples for Sequential Recommendation
Source: arXiv:2208.04116 source file (2022-08-08)
Supplement: Supplementary file 1 [file appendix_table_neg100.tex]

% Please add the following required packages to your document preamble:
% \usepackage{multirow}
% \usepackage[table,xcdraw]{xcolor}
% If you use beamer only pass "xcolor=table" option, i.e. \documentclass[xcolor=table]{beamer}
\begin{table*}[th]
\caption{Model performance of baselines and our proposed C$^2$-Rec are set with 100 negative items randomly sampled on four offline datasets, where `*' refers to modifying the original binary cross-entropy loss in SASRec with the training objective in recent baselines, e.g., CLRec, CL4SRec, StackRec. Our C$^2$-Rec is implemented on SASRec*. 
\textit{Improv.} and \textit{Improv.*} refer to the relative improvement of C$^2$-Rec over SASRec and SASRec*, respectively.}
\resizebox{\textwidth}{!}{
\begin{tabular}{lllllllllllll}
\toprule  
Datasets   & Metric & SASRec & SASRec* & GRU4Rec & BERT4Rec & TiSASRec & StackRec & CLRec  & CL4SRec & C$^2$-Rec  & Improv. & Improv.* \\
\hline
                         & HR@1    & 0.1845 & 0.1942  & 0.1075  & 0.0746   & 0.1779   & 0.1547   & 0.1351 & 0.2046  & {\textbf{0.2276}} & 23.36\% & 17.20\%  \\
                         & HR@5    & 0.3788 & 0.3551  & 0.2331  & 0.2189   & 0.3688   & 0.3341   & 0.2334 & 0.3819  & {\textbf{0.4064}} & 7.29\%  & 14.45\%  \\
                         & HR@10   & 0.4784 & 0.4420  & 0.3256  & 0.3157   & 0.4630   & 0.4399   & 0.2954 & 0.4750  & {\textbf{0.4939}} & 3.24\%  & 11.74\%  \\
                         & NDCG@5  & 0.2859 & 0.2783  & 0.1718  & 0.1480   & 0.2780   & 0.2477   & 0.1863 & 0.2971  & {\textbf{0.3218}} & 12.56\% & 15.63\%  \\
\multirow{-5}{*}{Beauty} & NDCG@10 & 0.3181 & 0.3064  & 0.2015  & 0.1792   & 0.3084   & 0.2819   & 0.2062 & 0.3272  & {\textbf{0.3500}} & 10.03\% & 14.23\%  \\
\hline
                         & HR@1    & 0.1678 & 0.1744  & 0.0866  & 0.0662   & 0.1501   & 0.1241   & 0.1331 & 0.1850  & {\textbf{0.1949}} & 16.15\% & 11.75\%  \\
                         & HR@5    & 0.3984 & 0.3776  & 0.2537  & 0.2217   & 0.3582   & 0.2993   & 0.3349 & 0.3965  & {\textbf{0.4186}} & 5.07\%  & 10.86\%  \\
                         & HR@10   & 0.5241 & 0.4910  & 0.3817  & 0.3525   & 0.4764   & 0.4156   & 0.4689 & 0.5115  & {\textbf{0.5360}} & 2.27\%  & 9.17\%   \\
                         & NDCG@5  & 0.2870 & 0.2796  & 0.1709  & 0.1440   & 0.2577   & 0.2138   & 0.2361 & 0.2949  & {\textbf{0.3112}} & 8.43\%  & 11.30\%  \\
\multirow{-5}{*}{Sport}  & NDCG@10 & 0.3276 & 0.3162  & 0.2121  & 0.1860   & 0.2959   & 0.2513   & 0.2793 & 0.3321  & {\textbf{0.3491}} & 6.56\%  & 10.40\%  \\
\hline
%                          & HR@1    & 0.3476 & 0.3709  & 0.2228  & 0.1205   & 0.2900   & 0.2599   & 0.3039 & 0.3783  & {\textbf{0.3826}} & 10.07\% & 3.15\%   \\
%                          & HR@5    & 0.6444 & 0.6283  & 0.4852  & 0.3601   & 0.5960   & 0.5113   & 0.5759 & 0.6385  & {\textbf{0.6554}} & 1.71\%  & 4.31\%   \\
%                          & HR@10   & 0.7450 & 0.7208  & 0.6089  & 0.5152   & 0.7167   & 0.6219   & 0.6846 & 0.7299  & {\textbf{0.7455}} & 0.07\%  & 3.43\%   \\
%                          & NDCG@5  & 0.5063 & 0.5086  & 0.3600  & 0.2417   & 0.4516   & 0.3922   & 0.4476 & 0.5177  & {\textbf{0.5290}} & 4.48\%  & 4.01\%   \\
% \multirow{-5}{*}{Video}  & NDCG@10 & 0.5390 & 0.5386  & 0.4001  & 0.2917   & 0.4908   & 0.4280   & 0.4829 & 0.5474  & {\textbf{0.5583}} & 3.58\%  & 3.66\%   \\
                         & HR@1    & 0.2511 & 0.2875  & 0.1349  & 0.1396   & 0.2549   & 0.1988   & 0.2281 & 0.2837  & {\textbf{0.3068}} & 22.18\% & 6.71\%   \\
                         & HR@5    & 0.6393 & 0.6339  & 0.4826  & 0.4758   & 0.6238   & 0.5285   & 0.6111 & 0.6350  & {\textbf{0.6683}} & 4.54\%  & 5.43\%   \\
                         & HR@10   & 0.8256 & 0.8008  & 0.7322  & 0.7255   & 0.8001   & 0.7034   & 0.8197 & 0.8039  & {\textbf{0.8340}} & 1.02\%  & 4.15\%   \\
                         & NDCG@5  & 0.4512 & 0.4674  & 0.3095  & 0.3082   & 0.4454   & 0.3675   & 0.4244 & 0.4657  & {\textbf{0.4951}} & 9.73\%  & 5.93\%   \\
\multirow{-5}{*}{Yelp}   & NDCG@10 & 0.5118 & 0.5215  & 0.3901  & 0.3888   & 0.5027   & 0.4241   & 0.4921 & 0.5206  & {\textbf{0.5489}} & 7.25\%  & 5.25\% \\
\hline
\multirow{5}{*}{WeChat} & HR@1    & 0.1836 & 0.2005  & 0.1218  & 0.1209   & 0.1971   & 0.1715   & 0.1585 & 0.2077  & \textbf{0.2213} & 20.53\% & 10.37\%  \\
                        & HR@5    & 0.5718 & 0.5903  & 0.4366  & 0.4435   & 0.5827   & 0.4688   & 0.4361 & 0.6049  & \textbf{0.6396} & 11.86\% & 8.35\%   \\
                        & HR@10   & 0.7114 & 0.7216  & 0.6021  & 0.6002   & 0.7063   & 0.6891   & 0.6351 & 0.7299  & \textbf{0.7862} & 10.51\% & 8.95\%   \\
                        & NDCG@5  & 0.4023 & 0.4182  & 0.2874  & 0.2931   & 0.4096   & 0.3622   & 0.3429 & 0.4291  & \textbf{0.4595} & 14.22\% & 9.87\%   \\
                        & NDCG@10 & 0.4528 & 0.4617  & 0.3465  & 0.3398   & 0.4511   & 0.4437   & 0.4017 & 0.4635  & \textbf{0.5080}  & 12.19\% & 10.07\%  \\
\bottomrule
\end{tabular}}
\end{table*}
